# Supplementary material for: Hierarchical Auto-Organizing System for Open-Ended Multi-Agent Navigation
Source: arXiv:2403.08282 source file (2024-03-18)
Supplement: Supplementary file 1 [file 6_appendix.tex]

\appendix

\setcounter{figure}{0}
\setcounter{table}{0}

\section{Centralized Planning with Decentralized Execution}\label{sec:CPDE}

Evoked from the Centralized Training with Decentralized Execution~(CTDE) framework for cooperative Multi-Agent Reinforcement Learning~(MARL), we propose Centralized Planning with Decentralized Execution~(CPDE) for the cooperative LLM-based Multi-Agent system. This architecture leverages global state information to inform the planning process, while the execution of tasks is carried out by local agents independently. CPDE is tailored to maximize the synergy of global oversight and local autonomy, ensuring efficient navigation and task completion in complex environments.

\paragraph{Centralized planning for manager agent.}

The centralized planning process for a manager agent simulates a high-level understanding like that of a human planner. The process includes understanding the environment's dynamic global states, recognizing the action agents' capabilities and limitations, and devising a strategy. It is equipped with a set of specialized modules, which are listed below:

\noindent \textbf{$\bullet$ Planner} $\mathcal{P}$ 
The planner module acts as the brain of the centralized planning process. It synthesizes global situational data to formulate comprehensive plans that align with the overarching objectives of the task. This module considers the full breadth of the environment, predicting potential outcomes and strategizing accordingly to optimize the path to success.

\noindent \textbf{$\bullet$ Describer} $\mathcal{D}_s$\label{sec:c_describer}
The describer module is essential given the vast multi-modal data available to the manager agent. It serves two crucial purposes: firstly, to distill the extensive data into a concise summary, making it more manageable and interpretable; secondly, to translate multimodal data into a textual format that can be efficiently stored and retrieved from memory, bridging the gap between visual information and linguistic representation.

\noindent \textbf{$\bullet$ Deployer} $\mathcal{D}_p$\label{sec:c_deployer} 
The deployer module actualizes the auto-organization principle at the managerial level, assigning key action agents to specific subtasks. It translates the centralized plan into actionable directives, ensuring that each agent understands its role and the expectations for its performance.

The process of subtask deployment can be conceptualized as follows:
\begin{equation}
T_{k} = \mathcal{D}_p(M, G_{m}, S_{m})
\end{equation}
where \( T_{k} \) is the task for the key action agent \( k \), \( M \) represents the multi-modal information, \( G_{m} \) is the goal provided by the main agent, and \( S_{m} \) is the suggested strategy for achieving \( G_{m} \).

\noindent \textbf{$\bullet$ Critic} $\mathcal{C}_r$\label{sec:c_critic} 
The critic module is an internal auditor for the planning and deployment processes. It evaluates the planner and deployer's decisions, providing feedback that can refine strategies and agent assignments. By continuously reviewing and critiquing the central plan and its execution, the critic ensures that the system remains robust and adaptable.

\paragraph{Decentralized execution for action agent.}

The decentralized execution process is designed to capitalize on the autonomy and flexibility of action agents. These agents navigate the environment, perform tasks, and learn from their interactions guided by the strategic direction from the centralized planning of the manager agent. It is empowered by modules which are listed below:

\noindent \textbf{$\bullet$ Actor} $\mathbf{A}$ 
At the decentralized level, the actor module is responsible for the concrete, code-driven execution of tasks. Utilizing GPT-4's capabilities, the actor translates strategic plans into executable code actions, such as navigating to specific environmental coordinates.

\noindent \textbf{$\bullet$ Deployer} $\mathbf{D}_p$ 
The deployer module within the action agent domain oversees the formation and adjustment of dynamic agent groups, mirroring its centralized counterpart in~\Cref{sec:c_deployer}. In addition, it also needs to complete the distribution of simple functions and distribute the simple instructions executed by this key action agent to all sub-agents. It ensures that the collective execution of tasks is coherent and aligned with the strategic directives of the manager agent.

This directive process can be formalized as:
\begin{equation}
C_{s} = \mathbf{D}_p(T_{k}, P_{k})
\end{equation}
where \( C_{s} \) represents the command for the sub-action agent \( s \), \( T_{k} \) is the task received from the key action agent, and \( P_{k} \) is the position or target information that differentiates the individual sub-agent tasks.

\noindent \textbf{$\bullet$ Curriculum} $\mathbf{C}_u$ 
The curriculum module facilitates continuous learning and adaptation for action agents. By engaging with a series of progressively complex tasks, agents refine their skills and strategies. This experiential learning is stored within the multimodal memory, contributing to the system's overall knowledge and expertise.

\noindent \textbf{$\bullet$ Skill} $\mathbf{S}$
The skill module refers to code database retrieval. As a repository of pre-coded strategies and actions, the skill database allows action agents to swiftly draw upon past experiences to address current challenges. This saves computational resources and streamlines the execution by applying proven solutions.

\noindent \textbf{$\bullet$ Critic} $\mathbf{C}_r$
The decentralized critic module is similar to its centralized counterpart in~\Cref{sec:c_critic}, providing ongoing evaluation and feedback. However, it reviews agents' actions and deployments, suggesting revisions to enhance performance and maintain alignment with the centralized plan.

\section{Multi-modal Information Platform}

The Multi-modal Information Platform is an advanced data processing hub designed to handle diverse types of information inputs and facilitate the interaction between humans and agents. This platform serves multiple critical functions: 

\noindent \textbf{$\bullet$} It is the initial point of contact for human interaction where the navigation goals are established; 

\noindent \textbf{$\bullet$} It acts as a dynamic repository for the state information of all agents, encompassing vision, textual descriptions, and audio logs; 

\noindent \textbf{$\bullet$} It maintains a dynamic map that reflects the exploration areas and updates from all action agents.

\paragraph{Navigation goal with human interaction.}
The platform is the interface for human operators, or automated rule sets to input initial navigation goals. These goals can be specified in various forms, such as visual objectives (image goals), textual objectives (object goals), or auditory cues (audio goals). The ability to accept multi-modal inputs allows for a high degree of flexibility and precision in defining the tasks for the agent system.

\noindent \textbf{$\bullet$ Image Goal}
The image goal represents visual objectives. It might be a specific location or item that the agents must locate within their environment. The platform processes these visual inputs and integrates them into the dynamic map, guiding the agents toward fulfilling these visual tasks.

\noindent \textbf{$\bullet$ Object Goal}
Textual or object goals are descriptive tasks processed by the platform to provide context and directives to the agents. These are translated into actionable items for the agents to execute, aligning with the overall mission objectives set by human operators or pre-defined rules.

\noindent \textbf{$\bullet$ Audio Goal}
Audio goals are auditory cues that can trigger specific behaviors or guide agents towards areas of interest. The platform's ability to process and interpret audio inputs adds layer of interaction and task specification for the agents.

\paragraph{Dynamic state storage.}
Central to the platform's functionality is its capacity to store and update the dynamic state of each agent. This includes a continuous feed of sensory inputs like vision and audio and textual logs that describe the agents' perceptions and actions. This real-time data is crucial for the system to adapt and respond to the changing environment and the agents' experiences.

This component deals with the sensory data collected by the agents. Vision and audio states are continuously fed into the platform, updating the system's understanding of the environment and influencing the planning and execution processes.

\paragraph{Dynamic Map}
The dynamic map visually represents the exploration domain, showcasing only the areas the agents have explored. It is updated in real-time with information from all action agents, providing a strategic overview of the environment. This map is instrumental in planning and executing navigation tasks as it reflects the current knowledge and discoveries made by the agent collective.

The following equations can formalize the dynamic map's function:

\begin{equation}
    M_t = M_{t-1} \cup \bigcup_{i=1}^{n}S_{i,t}
\end{equation}

\begin{equation}
    S_{i,t} = F(V_{i,t}, A_{i,t})
\end{equation}

Where \( M_t \) represents the dynamic map at time \(       Q  t \), \( S_{i,t} \) is the state information from agent \( i \) at time \( t \), including both visual \( V_{i,t} \) and audio \( A_{i,t} \) data. \( F \) is the function that integrates the sensory data into the map, and \( n \) is the number of active agents. This real-time updating mechanism ensures that the dynamic map remains an accurate and current representation of the exploration field.

\section{Communication in Multi-Agent Systems}

Effective communication is meticulously orchestrated to ensure cohesive operation and efficient task completion. This involves a dual-layered communication strategy: one between the main agent and key action agents and another between key action agents and their respective sub-action agents.

\paragraph{Main agent-Key action agent communication.}

The communication between the main agent and key action agents is bidirectional and critical for the delegation and execution of tasks. The main agent is responsible for deploying subtasks, which include detailed multi-modal targets to the key action agents. These targets may encompass a variety of sensory data, such as visual and auditory information, accompanied by textual suggestions that guide the method of achieving the target and specify the quantity of the targets to be engaged.

Once a key action agent receives its subtask, it processes the multi-modal information provided by the main agent, translating it into a simplified action plan. This plan is then further distilled into the simplest possible set of commands to be executed by the sub-action agents. The key action agent also determines the number of sub-action agents required to efficiently achieve the goal, ensuring that resources are allocated appropriately.

\paragraph{Intra-Key action agent communication.}

The key action agent acts as the central command for its group of sub-action agents. It communicates the simplified action steps to each sub-agent, who will execute the task. While all sub-action agents within a group work towards a common objective, they are assigned distinct targets to maximize efficiency and coverage. For instance, in a scenario where the goal is to explore chests, each sub-agent would be directed to a different location to avoid redundancy and potential conflicts.

Sub-action agents receive their directives as precise and uncomplicated commands, ensuring clarity and ease of execution. The commands are designed to be directly actionable, allowing sub-action agents to perform tasks without the need for further interpretation or decision-making.

\section{Model Initial}

Initially, no status information is available since the conductor has not been created yet. Therefore, the formulation is different. Given any goal $g$ in $\mathcal{G}=\{Im, Oj, Au \}$, the manager agent~$M$ oversees the initial global environment with the initial dynamic map $\mathcal{M}_0$. Then, it plans the initial sub-goal list $G^s = \{g^s_i\}_{i\leq N}$ and assigns these subtasks to the conductor list $C =\{c_i\}_{i\leq N}$ with the initial state list $S =\{s_i\}_{i\leq N}$ based on this. Then, the first action $\mathbf{a}^{c}_i$ of the conductor can be obtained as follows,

\begin{equation}
\mathbf{a}^c_i = \mathbf{MLM}^C(g^s_i, s^0_i), \qquad g^s_i \in G^s = \mathbf{MLM}^M(g,\mathcal{M}_0), 
\end{equation}

After completing the corresponding sub-goal $g^s_i$, the manager agent can allocate a new sub-goal by combining the current status information through ~\Cref{eqn:main_function}. The process will continue until the entire goal is achieved. 

\section{Map Exploration}
\begin{figure*}[h]
% \vspace{-30pt}
% \setlength{\tabcolsep}{1.5pt}
\centering
    \includegraphics[width=\linewidth]{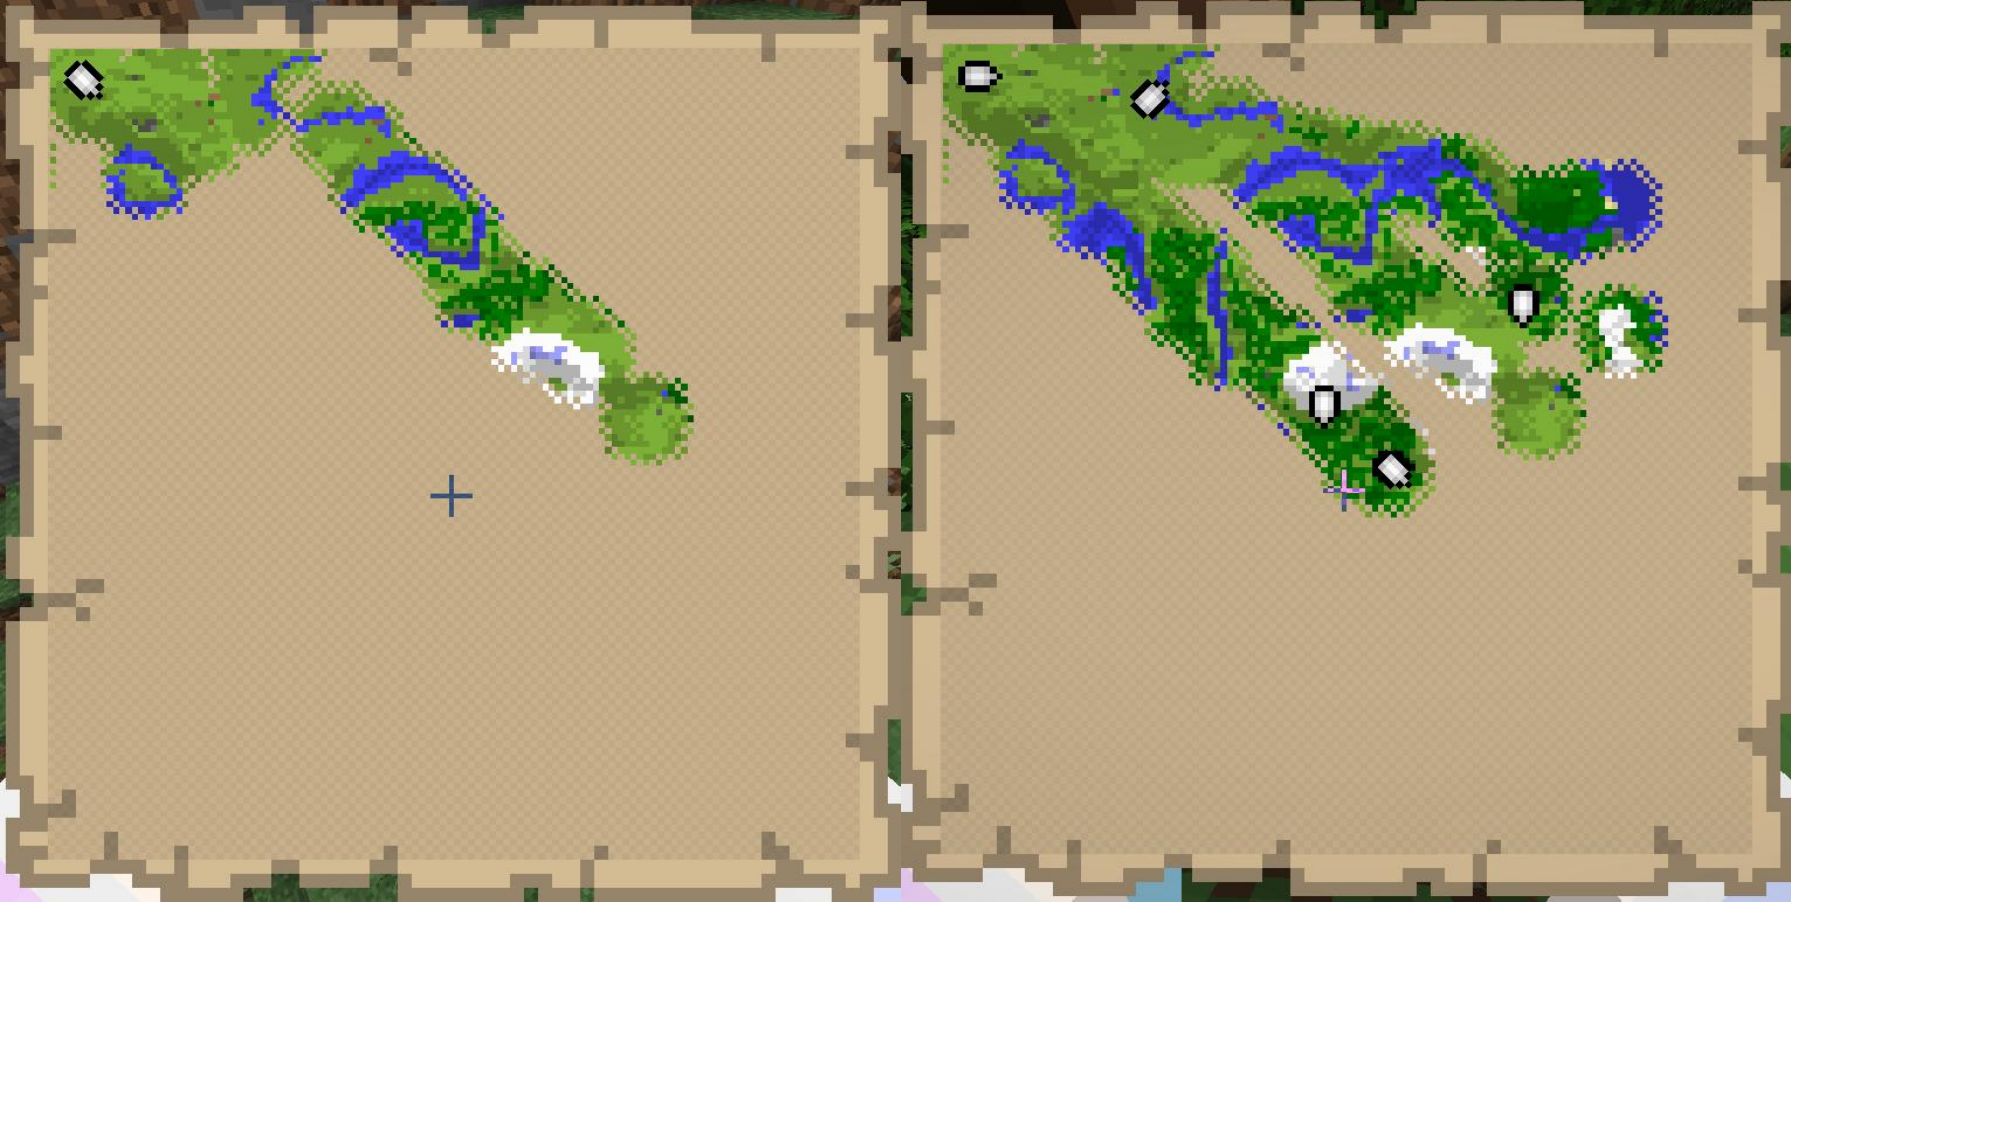}\\
    % \vspace{-5pt}
    \caption{\small \textbf{Map exploration.} 
    }
    \label{fig:map_explore}
\end{figure*}

\subsection{Curriculum Upgrading Agents}\label{sec:upgrading}

\paragraph{Curriculum learning with memory.} 
The problem now is determining the source of the multi-modal memory mentioned earlier. To address this, we take inspiration from the lifelong learning strategy used in many reinforcement learning problems~\citep{wang2023voyager}, both in close-world and open-world settings. 
First, we generate a set of tasks that act as a curriculum for agents to explore the world. During this process, HAS creates plans, interacts with the environment, learns from errors, and stores all these experiences in memory. 
Then, we test HAS on various navigation tasks following this learning phase. HAS can produce more effective plans by combining its memory with its planning experiences.

\paragraph{Continous learning with summarization.}~\label{para:COS}
We have noticed that the learning process, where the memory is being filled, can continue throughout the gameplay. The agent can gradually acquire more skills as the gameplay progresses and more experiences are gained. However, as the memory gets larger, challenges such as difficulty arise, such as understanding the game's situation and slow interaction speed. We implement the Chain of Summarization method~\citep{ma2023large} to tackle these challenges.
